# Supplementary material for: InstructEdit: Instruction-based Knowledge Editing for Large Language Models
Source: arXiv:2402.16123 source file (2024-04-28)
Supplement: Supplementary file 1 [file appendix.tex]

\section{Experimental details}
We utilize Pytorch to conduct experiments on a single A800 GPU.
The number of edit is set to 1.
The max sequence length is set to 96.
\text{\ours} and MEND's optimizations are performed using the Adam optimizer, while KnowledgeEditor (KE) utilizes Adamw, and FT-L and CaliNet employ AdaFactor.
Layer normalization $\epsilon$ is set to 1e-1 across all modules2. 
Grid search is used for hyperparameter tuning, and the best hyperparameters are in Table \ref{tab:hyper}.

\begin{table}[!b]
\centering
\small
\resizebox{1.0\columnwidth}{!}{
\resizebox{0.5\textwidth}{!}{% <------ Don't forget this %
\begin{tabular}{lcccccccc}
\toprule
              % &         \multicolumn{4}{c}{\bf FB15k-237}                           &        \multicolumn{4}{c}{\bf WN18RR}                           \\ \cmidrule(lr){2-5}                         \cmidrule(lr){6-9}   
Type  & Ours & MEND & KE & CaliNet \\
\midrule
% \rule{0pt}{15pt}
Edit Num     & 1 & 1 & 1 & 1 \\
% \rule{0pt}{15pt}
Steps    &  5k & 5k & 10k & 15k \\
Accumulate    &  2 & 2 & 2 & 2 \\
Learning Rate    &  1e-6 & 1e-6 & 1e-5 & 5e-4 \\
\bottomrule
\end{tabular}
}%
}
\caption{
The best hyperparameters.
}
\label{tab:hyper}
\end{table}

\begin{table}[!b]
\centering
\small
\resizebox{1.0\columnwidth}{!}{
\resizebox{0.5\textwidth}{!}{% <------ Don't forget this %
\begin{tabular}{lcccccccc}
\toprule
              % &         \multicolumn{4}{c}{\bf FB15k-237}                           &        \multicolumn{4}{c}{\bf WN18RR}                           \\ \cmidrule(lr){2-5}                         \cmidrule(lr){6-9}   
Type  & \wikicf & \wikirecent & \convsent & \zsre \\
\midrule
% \rule{0pt}{15pt}
Train     & 1,427 & 570 & 14,390 & - \\
% \rule{0pt}{15pt}
Test    &  839 & 1,266 & 800 & 1,037 \\
\bottomrule
\end{tabular}
}%
}
\caption{
The statistics of datasets.
}
\label{tab:dataset}
\end{table}

\section{Datasets Details}

Table \ref{tab:dataset} presents the dataset statistics, including the original count of \text{\convsent}. 
However, the body of the paper focuses on a subset of \text{\convsent} that have been balanced to ensure a fair training process, which is reflected in the main findings.
The balanced \text{\convsent} is used for training in the main results presented in the paper. 
Notably, The training process for the \text{\convsent} is described as being consistent with the original setting, particularly in terms of loss calculation. 
It requires inputting a specific number of sentences into the model, which demands a significant amount of VRAM. 
Due to the high VRAM requirements, we do not conduct experiments on the \text{\convsent} dataset using the LLaMA model. 
While the training process for \text{\convsent} remains the same, the evaluation method has been slightly modified; inputs concerning Reliability and Locality are matched to form 10 unique test cases, which are then assessed individually with their performance averaged to yield the overall results.

\section{Case Study}
In the case of the dataset \text{\wikicf}, when prompted with the query ``The name of the spouse of James R. Jordan, Sr. is?'' with the target response being ``Zhang You''.
Prior to editing, the model's response is ``James''. 
The model, edited by MEND, incorrectly answers ``James You'' while \text{\ours} with instruction correctly identifies ``Zhang You''.
In the case of the hold out dataset \text{\zsre}, when prompted with the query ``What is the native tongue of Pierre Corneille?'' with the target response being ``German''.
Prior to editing, the model's response is a blank space. 
The model, edited by MEND, incorrectly answers ``French'' while \text{\ours} correctly identifies ``German''.
